# Supplementary material for: Towards Low-Energy Adaptive Personalization for Resource-Constrained Devices
Source: arXiv:2403.15905 source file (2024-03-29)
Supplement: Supplementary file 1 [file 8-Appendix.tex]

\newpage
\onecolumn
\begin{appendix}
\section{Appendix} 
\label{sec:appendix}

\begin{table}[]
\begin{tabular}{ccccccc}
\hline
Training Size &
  Block 1 &
  Block 2 &
  Block 3 &
  FC &
  Block Avg &
  Full \\ \hline
10\% &
  \cellcolor[HTML]{FFFFFF}15.94±0.98 &
  \cellcolor[HTML]{FFFFFF}29.78±0.34 &
  \cellcolor[HTML]{FFFFFF}54.20±0.28 &
  \cellcolor[HTML]{FFCC67}84.43±0.10 &
  46.08±0.24 &
  50.86±0.35 \\
20\% &
  \cellcolor[HTML]{FFFFFF}21.95±1.05 &
  \cellcolor[HTML]{FFFFFF}40.32±0.59 &
  \cellcolor[HTML]{FFFFFF}66.84±0.38 &
  \cellcolor[HTML]{FFCC67}84.87±0.17 &
  53.65±0.41 &
  62.65±0.27 \\
30\% &
  \cellcolor[HTML]{FFFFFF}25.87±0.68 &
  \cellcolor[HTML]{FFFFFF}45.98±0.40 &
  \cellcolor[HTML]{FFFFFF}71.78±0.43 &
  \cellcolor[HTML]{FFCC67}84.91±0.20 &
  57.14±0.16 &
  69.81±0.45 \\ \hline
\end{tabular}
\end{table}

\end{appendix}
